# Supplementary material for: Adapting a Kidney Exchange Algorithm to Align with Human Values
Source: arXiv:2005.09755 source file (2020-05-19)

# Adapting a Kidney Exchange Algorithm to Align with Human Values
## Appendix: Additional Experimental Methods and Results

<u>Selecting Attributes</u>

After a short description of how kidney exchanges work, participants were asked:

"Suppose a country is starting up a kidney allocation system, in which people who need a kidney transplant from a stranger are kept on a waiting list. Every time a kidney is donated to the system, it is given to one of the people on the list. The country wants to develop a clear policy to determine who on the list should receive each donated kidney. For example, some of their citizens want the policy to prioritize younger recipients, while others want it to prioritize older ones, and still others think that age shouldn't be taken into account at all. What factors do you think the policy *should* take into account? What factors do you think it would be *morally wrong* for the policy to take into account?" Participants were then given space to fill in as many factors as they wished, and given the opportunity to enter text about why each factor should be included or excluded from the policy.

100 participants' responses were scored by two independent experimenters into the categories provided in Supplementary Table 1 after qualitative examination of the full range of responses. The number of times each factor was mentioned in a response was tallied.

Supplementary Table 1: Attribute Frequencies

| **Factor or Attribute** | **Total Frequency** | **% Positive (% who said factor should vs. should not be taken into account)** |
|---|---|---|
| Age | 91 | 89% |
| Ability to pay | 83 | 7% |
| Race | 74 | 0% |
| Health - Behavioral | 58 | 91% |
| Health-Unrelated | 53 | 83% |
| Sex/Gender | 48 | 10% |
| Personal Beliefs | 43 | 0% |
| Social Standing | 38 | 8% |
| Sexual Orientation | 28 | 0% |
| Dependents | 23 | 78% |
| Occupation | 18 | 39% |
| Citizenship | 11 | 9% |
| Nepotism | 12 | 0% |
| Criminal Record | 14 | 71% |
| Societal Contribution | 10 | 70% |
| Intelligence/Education | 8 | 13% |
| Quantity/Quality of Life | 9 | 89% |
| Mental Factors | 6 | 100% |
| Location | 6 | 0% |

Experiment 3: Varying Bradley-Terry Scores

In addition to the weights and alternative weights described in the main text of the manuscript, we also ran simulations with the weight vectors listed in Supplementary Table 2.

Supplementary Table 2: Alternate Weight Vectors

| Name | Description | Profile Weight (rounded to 3 decimal places) | | | | | | | |
|---|---|---|---|---|---|---|---|---|---|
| | | 1 | 2 | 3 | 4 | 5 | 6 | 7 | 8 |
| Broad | same order; larger constant intervals | 1 | 0.800 | 0.900 | 0.600 | 0.700 | 0.400 | 0.500 | 0.300 |
| Linear Prioritized | same order; small constant intervals | 1 | 0.998 | 0.999 | 0.996 | 0.997 | 0.994 | 0.995 | 0.993 |
| Predictors | B-T weights, attribute-based | 1 | 0.131 | 0.291 | 0.038 | 0.089 | 0.011 | 0.026 | 0.003 |
| Reverse_ Diff | reversed differences | 1 | 0.979 | 0.991 | 0.933 | 0.967 | 0.766 | 0.900 | 0.003 |
| (Original) Prioritized | B-T weights, direct | 1 | 0.103 | 0.236 | 0.036 | 0.07 | 0.011 | 0.024 | 0.003 |
| Standard | all equal | 1 | 1 | 1 | 1 | 1 | 1 | 1 | 1 |

There was very little difference in the matchings produced by each of these weight vectors, as illustrated below:

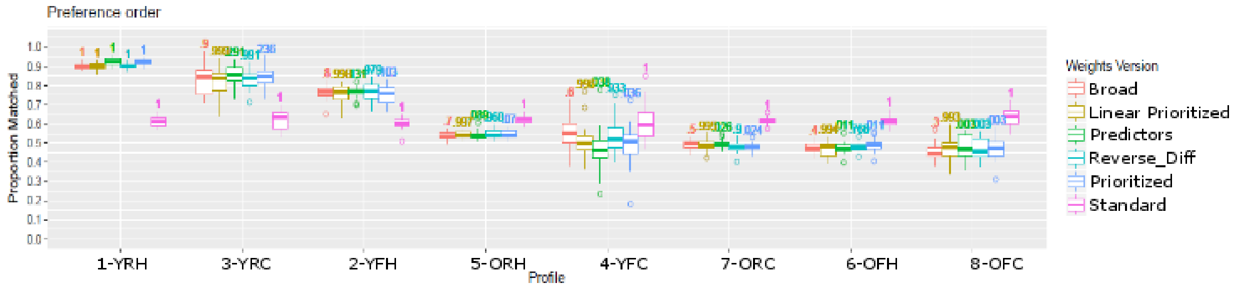

Supplement: Supplementary file 1 [file appendix.pdf]
